# Supplementary material for: Local Convergence Properties of SAGA/Prox-SVRG and Acceleration
Source: arXiv:1802.02554 source file (2018-11-01)
Supplement: Supplementary file 1 [file sec-appendix.tex]

\section{Riemannian Geometry}

% In this part, we introduce some result of the Riemannian geometry.
We denote $\calM$ a $C^2$-smooth submanifold of $\bbR^n$.
%, meaning that for a given point $x \in \calM$, there exists a local function $\chi: \bbR^n \to \bbR^l$ around $x$ such that $\chi$ is $C^2$-smooth.
% 
We also denote $\tanSp{\Mm}{x}$ the tangent space of $\Mm$ at a point $x$, and $\normSp{\Mm}{x}$ the normal space.
In the following, we present some preliminaries on the Riemannian geometry.

\subsection{Exponential map}

Given two points $x, x' \in \calM$, define $\mathfrak{g}(t;x, h), t \in [0,1]$ their geodesics with
\[
\mathfrak{g}(0;x, h) = x  ,~~
\mathfrak{g}(1;x, h) = x  ~~ \textrm{and}~~
\dot{\mathfrak{g}}(t;x, h) = h , \forall t \in [0,1]  ,
\]
that $\mathfrak{g}$ has constant \emph{velocity} along the geodesic.
or every $h \in \tanSp{\calM}{x}$, there exists an interval $\calI$ about $0$ and a unique geodesic $\mathfrak{g}(t;x, h): \calI \to \calM$ such that $\mathfrak{g}(0; x, h) = x$ and $\dot{\mathfrak{g}}(0;x, h) = h$.
The mapping
  \[
  \begin{aligned}
  \Exp_x 
  &: \tanSp{\calM}{x} \to  \calM \\
  &: h \mapsto \Exp_{x}(h) =  \mathfrak{g}(1;x, h) ,
  \end{aligned}
  \]
is called \emph{Exponential map}.
Given $x, x' \in \calM$, the direction $h$ we are interested in is such that 
\[
\Exp_x(h) = x' = \mathfrak{g}(1;x, h)  .
\]

\subsection{Parallel translation}

Given two points $x, x' \in \calM$, let $\tanSp{\calM}{x}, \tanSp{\calM}{x'}$ be their corresponding tangent spaces. Define 
\[
\tau : \tanSp{\calM}{x} \to \tanSp{\calM}{x'} ,
\]
the parallel translation along the unique geodesic joining of $x$ and $x'$, which is isomorphism and isometry w.r.t. the Riemannian metric.

\subsection{Riemannian covariant gradient and Hessian}

Given a function $\Phi$ which is $C^2$ along the manifold $\calM$, then its Riemannian (covariant) gradient at $x \in \calM$ is the vector $\nabla_{\calM} \Phi(x) \in \tanSp{\calM}{x}$ defined by
\[
\iprod{\nabla_{\calM} \Phi(x)}{h} = \qfrac{d}{dt} \Phi\Pa{\proj_{\calM}(x+th)}\big|_{t=0} ,~~ \forall h \in \tanSp{\calM}{x},
\]
where $\proj_{\calM}$ is the projection operator onto $\calM$. %, and $\tanSp{\calM}{x}$ can be replaced by $\TJ{x}$ owing to the local normal sharpness property. 
The Riemannian (covariant) Hessian of $\Phi$ at $x$ is the symmetric linear mapping $\nabla^2_{\calM} \Phi(x)$ from $\tanSp{\calM}{x}$ to itself which is defined as
\beq\label{eq:rh}
\iprod{\nabla^2_{\calM} \Phi(x) h}{h} = \qfrac{d^2}{dt^2} \Phi\Pa{\proj_{\calM}(x+th)}\big|_{t=0} ,~~ \forall h \in \tanSp{\calM}{x} .
\eeq
This definition agrees with the usual definition using geodesics or connections.

Further more, according to \cite{absil2013extrinsic}, given $x \in \calM$ and a direction $h \in \tanSp{\calM}{x}$, the Riemannian Hessian of $\Phi$ at $x$ can be also written as
\beq\label{eq:rh-wgtmap}
\nabla^2_{\calM} \Phi(x) h = \PT{\tanSp{\calM}{x}} \nabla^2 \widetilde{\Phi}(x) h + \mathfrak{W}_{x}\Pa{h, \PT{\normSp{\calM}{x}}\nabla \widetilde{\Phi}(x)}  ,
\eeq
where $\mathfrak{W}(\cdot, \cdot)$ is the Weingarten map at $x$ \cite{chavel2006riemannian}, $\widetilde{\Phi}$ is the smooth representation of $\Phi$ along $\calM$ near $x$.

For our problem in consideration \eqref{eq:min-Phi}, given a point $x \in \calM$, \emph{if $R \in \PSF{x}{\calM}$ and $F$ locally $C^2$-smooth around $x$}, then owing to the smooth perturbation rule of partly smooth function \cite[Corollary 4.7]{Lewis-PartlySmooth}, we have also $\Phi \in \PSF{x}{\calM}$.
In the lemma below we show positive semi-definiteness of the Riemannian Hessian of $\Phi$ under partial smoothness.

\begin{lemma}\label{lem:riemhesspsd} 
For problem \eqref{eq:min-Phi}, let condition \iref{A:R}-\iref{A:minimizers-nonempty} hold. Suppose there exists a $\xbar \in \bbR^n$ such that $R \in \PSF{\xbar}{\calM}$, $F$ is locally $C^2$ around $\xbar$, and moreover $-\nabla F(\xbar) \in \ri\Pa{\partial R(\xbar)}$.
 %
 % Define function $\Psi(x) = R(x) + \iprod{x}{\nabla F(\xbar)}$, then the Riemannian Hessian of $\Psi$ at $\xbar$ is \emph{positive semi-definite}, namely, 
 Then for any $h \in \tanSp{\calM}{\xbar}$,
 \[
 \iprod{\PT{\tanSp{\calM}{\xbar}} \nabla^2 \widetilde{R}(\xbar) h + \mathfrak{W}_{\xbar}\Pa{h, \PT{\normSp{\calM}{\xbar}}(\nabla \widetilde{R}(\xbar) + \nabla F(\xbar))} h}{h} \geq 0  .
 \]
 \end{lemma}
 \begin{proof}
First we have $\Phi \in \PSF{\xbar}{\calM}$. 
Define $\Psi(x) = R(x) + \iprod{x}{\nabla F(\xbar)}$, 
from \eqref{eq:rh-wgtmap}, the Riemannian Hessian of $\Psi$ at $\xbar$ along direction $h \in \tanSp{\calM}{\xbar}$ reads,
\[
\begin{aligned}
\nabla^2_{\calM} \Psi(\xbar) h
&= \PT{\tanSp{\calM}{\xbar}} \nabla^2 \widetilde{\Psi}(\xbar) h + \mathfrak{W}_{\xbar}\Pa{h, \PT{\normSp{\calM}{\xbar}}\nabla \widetilde{\Psi}(\xbar)}  \\
&= \PT{\tanSp{\calM}{\xbar}} \nabla^2 \widetilde{R}(\xbar) h + \mathfrak{W}_{\xbar}\Pa{h, \PT{\normSp{\calM}{\xbar}}(\nabla \widetilde{R}(\xbar) + \nabla F(\xbar))}  .
\end{aligned}
\]
Since also $\Psi(x) = R(x) - \iprod{x}{-\nabla F(\xbar)}$ and $-\nabla F(\xbar) \in \ri\Pa{\partial R(\xbar)}$, then by \cite[Corollary 5.4]{LewisPartlyTiltHessian} and local normal sharpness, we have
\[
 \partial^2 R\Pa{\xbar|-\nabla F(\xbar)} h =
 \left\{
 \begin{aligned}
 	\nabla^2_{\calM} \Psi(\xbar) h    ,~~& h \in \tanSp{\calM}{\xbar}  , \\
 	\emptyset ,~~& h \notin \tanSp{\calM}{\xbar}  ,
 \end{aligned}  
 \right.
\]
 then applying \cite[Theorem 2.1]{poliquin1998tilt} leads to the claimed result.
 \end{proof}

We have the following lemma characterising the parallel translation and the Riemannian Hessian of two close points in $\calM$.

\begin{lemma} \label{lem:parallel-translation}
Let $x, x'$ be two close points in $\calM$, denote $\tanSp{\calM}{x}, \tanSp{\calM}{x'}$ be the tangent spaces of $\calM$ at $x, x'$ respectively, and $\tau : \tanSp{\calM}{x} \to \tanSp{\calM}{x'}$ be the parallel translation along the unique geodesic joining from $x$ to $x'$, then for the parallel translation we have
\[
\pa{\tau^{-1}\proj_{\tanSp{\calM}{x'}} - \proj_{\tanSp{\calM}{x}}}(x-x') = o(\norm{x'-x})  .
\] 
The Riemannian Taylor expansion of $\Phi$ at $x$ for $x'$ reads,
\beq\label{eq:taylor-expn}
\tau^{-1} \nabla_{\calM} \Phi(x') = \nabla_{\calM} \Phi(x) + \nabla^2_{\calM} \Phi(x)\proj_{\tanSp{\calM}{x}}(x'-x) + o(\norm{x'-x})  .
\eeq
\end{lemma}

\begin{proof}
From \cite[Chapter 5]{absil2009optimization}, we have that locally for two close points $x,x'$ in $\calM$
\[
\tau^{-1} = \PT{\tanSp{\calM}{x}} + o(\norm{x-x'}) ,
\]
also locally near $x$ along $\calM$, the operator $\PT{\tanSp{\calM}{x}}$ is $C_1$-smooth, hence
\[
\begin{aligned}
\lim_{x'\to x} \frac{ \norm{\pa{\tau^{-1}\proj_{\tanSp{\calM}{x'}} - \proj_{\tanSp{\calM}{x}}}(x-x')} }{ \norm{x-x'}}
&\leq \lim_{x'\to x} \frac{ \norm{\proj_{\tanSp{\calM}{x}}\pa{\proj_{\tanSp{\calM}{x'}} - \proj_{\tanSp{\calM}{x}}} } \norm{x-x'} }{ \norm{x-x'}} + o(\norm{x-x'})  \\
&\leq \lim_{x'\to x} \norm{\proj_{\tanSp{\calM}{x'}} - \proj_{\tanSp{\calM}{x}}} + o(\norm{x-x'}) = 0  .
\end{aligned}
\]
Since $x, x' \in \calM$ are close enough, then the Taylor expansion \cite[Remark 4.2]{smith1994optimization} of $\nabla_{\calM} \Phi$ of $x'$ at $x$ is
\beq\label{eq:taylor-expn-1}
\tau^{-1} \nabla_{\calM} \Phi(x') = \nabla_{\calM} \Phi(x) + \nabla^2_{\calM} \Phi(x)\Exp_x(h) + o(\norm{h})  .
\eeq
Moreover, owing to \cite[Lemma 5.1]{liang2014local} and , we have
\[
x' = \Exp_{x}(h) 
\proj_{\calM}(x+h) + o(\norm{h}^2)
 + o(\norm{h}) + o(\norm{h}^2)
 + o(\norm{h}) ,
\]
back to \eqref{eq:taylor-expn-1} we get
\[
\tau^{-1} \nabla_{\calM} \Phi(x') = \nabla_{\calM} \Phi(x) + \nabla^2_{\calM} \Phi(x)\proj_{\tanSp{\calM}{x}}(x'-x) + o(\norm{x'-x})  ,
\]
which is the claimed result.
\end{proof}
